# Supplementary material for: Efficient Off-Policy Learning for High-Dimensional Action Spaces
Source: arXiv:2403.04453 source file (2025-02-17)
Supplement: Supplementary file 1 [file aggregated_iqm.tex]

% This file was created with tikzplotlib v0.10.1.
\begin{tikzpicture}
\tikzstyle{every node}'=[font=\sffamily\scriptsize] 
\pgfplotsset{every tick label/.append style={font=\tiny}}

\begin{axis}[
legend cell align={left},
legend style={
  fill opacity=0.8,
  draw opacity=1,
  text opacity=1,
  at={(0.97,0.03)},
  anchor=south east,
  draw=lightgray204
},
width=\textwidth,
height=4cm,
xlabel shift=-0.2cm,
ylabel shift=-0.15cm,
title style={yshift=-0.25cm},
title={MyoSuite - MyoHand},
tick align=outside,
tick pos=left,
x grid style={darkgray176},
scaled x ticks=false,
xticklabels={,0,1,2,3,4,5},
xlabel={Env. Steps $(\times 10^6)$},
xmajorgrids,
xmin=-100000, xmax=5100000,
xtick style={color=black},
xtick={0,1000000,2000000,3000000,4000000,5000000},
xticklabels={0,1,2,3,4,5},
y grid style={darkgray176},
scaled y ticks=false,
ylabel={Success},
ymajorgrids,
ymin=-0.043275, ymax=1,
ytick style={color=black}
]

\path [draw=C1, fill=C1, opacity=0.2]
(axis cs:0,0)
--(axis cs:0,0)
--(axis cs:100000,0)
--(axis cs:200000,0)
--(axis cs:300000,0)
--(axis cs:400000,0)
--(axis cs:500000,0)
--(axis cs:600000,0.004)
--(axis cs:700000,0.0409)
--(axis cs:800000,0.02)
--(axis cs:900000,0.03045)
--(axis cs:1000000,0.07645)
--(axis cs:1100000,0.04625)
--(axis cs:1200000,0.088)
--(axis cs:1300000,0.0849)
--(axis cs:1400000,0.06535)
--(axis cs:1500000,0.1069)
--(axis cs:1600000,0.0529)
--(axis cs:1700000,0.06045)
--(axis cs:1800000,0.0976)
--(axis cs:1900000,0.076)
--(axis cs:2000000,0.184)
--(axis cs:2100000,0.1476)
--(axis cs:2200000,0.13295)
--(axis cs:2300000,0.21735)
--(axis cs:2400000,0.15645)
--(axis cs:2500000,0.1109)
--(axis cs:2600000,0.1749)
--(axis cs:2700000,0.1585)
--(axis cs:2800000,0.1616)
--(axis cs:2900000,0.17695)
--(axis cs:3000000,0.1669)
--(axis cs:3100000,0.1496)
--(axis cs:3200000,0.1616)
--(axis cs:3300000,0.11845)
--(axis cs:3400000,0.1285)
--(axis cs:3500000,0.11025)
--(axis cs:3600000,0.22135)
--(axis cs:3700000,0.1978)
--(axis cs:3800000,0.1909)
--(axis cs:3900000,0.1789)
--(axis cs:4000000,0.18715)
--(axis cs:4100000,0.16895)
--(axis cs:4200000,0.1049)
--(axis cs:4300000,0.1238)
--(axis cs:4400000,0.0818)
--(axis cs:4500000,0.1949)
--(axis cs:4600000,0.1847)
--(axis cs:4700000,0.17045)
--(axis cs:4800000,0.15025)
--(axis cs:4900000,0.1369)
--(axis cs:5000000,0.12445)
--(axis cs:5000000,0.23575)
--(axis cs:5000000,0.23575)
--(axis cs:4900000,0.2531)
--(axis cs:4800000,0.3031)
--(axis cs:4700000,0.26175)
--(axis cs:4600000,0.3)
--(axis cs:4500000,0.30665)
--(axis cs:4400000,0.22575)
--(axis cs:4300000,0.2686)
--(axis cs:4200000,0.2231)
--(axis cs:4100000,0.3102)
--(axis cs:4000000,0.3151)
--(axis cs:3900000,0.288)
--(axis cs:3800000,0.30955)
--(axis cs:3700000,0.292)
--(axis cs:3600000,0.3231)
--(axis cs:3500000,0.28065)
--(axis cs:3400000,0.276)
--(axis cs:3300000,0.25865)
--(axis cs:3200000,0.3053)
--(axis cs:3100000,0.26265)
--(axis cs:3000000,0.322)
--(axis cs:2900000,0.29375)
--(axis cs:2800000,0.28865)
--(axis cs:2700000,0.3664)
--(axis cs:2600000,0.2691)
--(axis cs:2500000,0.2782)
--(axis cs:2400000,0.27085)
--(axis cs:2300000,0.3482)
--(axis cs:2200000,0.26065)
--(axis cs:2100000,0.2835)
--(axis cs:2000000,0.3115)
--(axis cs:1900000,0.19555)
--(axis cs:1800000,0.1931)
--(axis cs:1700000,0.15595)
--(axis cs:1600000,0.18995)
--(axis cs:1500000,0.22355)
--(axis cs:1400000,0.1642)
--(axis cs:1300000,0.2213)
--(axis cs:1200000,0.2106)
--(axis cs:1100000,0.11955)
--(axis cs:1000000,0.17175)
--(axis cs:900000,0.12955)
--(axis cs:800000,0.08155)
--(axis cs:700000,0.12175)
--(axis cs:600000,0.044)
--(axis cs:500000,0.00755)
--(axis cs:400000,0)
--(axis cs:300000,0)
--(axis cs:200000,0)
--(axis cs:100000,0)
--(axis cs:0,0)
--cycle;

\path [draw=C0, fill=C0, opacity=0.2]
(axis cs:0,0)
--(axis cs:0,0)
--(axis cs:100000,0)
--(axis cs:200000,0)
--(axis cs:300000,0)
--(axis cs:400000,0)
--(axis cs:500000,0)
--(axis cs:600000,0)
--(axis cs:700000,0)
--(axis cs:800000,0)
--(axis cs:900000,0)
--(axis cs:1000000,0)
--(axis cs:1100000,0.00245)
--(axis cs:1200000,0.000450000000000002)
--(axis cs:1300000,0.01245)
--(axis cs:1400000,0.01535)
--(axis cs:1500000,0.0449)
--(axis cs:1600000,0.08135)
--(axis cs:1700000,0.0776)
--(axis cs:1800000,0.09735)
--(axis cs:1900000,0.23245)
--(axis cs:2000000,0.28935)
--(axis cs:2100000,0.21725)
--(axis cs:2200000,0.37045)
--(axis cs:2300000,0.3136)
--(axis cs:2400000,0.3878)
--(axis cs:2500000,0.3858)
--(axis cs:2600000,0.43495)
--(axis cs:2700000,0.4758)
--(axis cs:2800000,0.51045)
--(axis cs:2900000,0.4509)
--(axis cs:3000000,0.586)
--(axis cs:3100000,0.56715)
--(axis cs:3200000,0.5316)
--(axis cs:3300000,0.59735)
--(axis cs:3400000,0.60445)
--(axis cs:3500000,0.5836)
--(axis cs:3600000,0.61335)
--(axis cs:3700000,0.6589)
--(axis cs:3800000,0.618)
--(axis cs:3900000,0.61715)
--(axis cs:4000000,0.6665)
--(axis cs:4100000,0.6863)
--(axis cs:4200000,0.73645)
--(axis cs:4300000,0.68005)
--(axis cs:4400000,0.724)
--(axis cs:4500000,0.6789)
--(axis cs:4600000,0.7525)
--(axis cs:4700000,0.8)
--(axis cs:4800000,0.7354)
--(axis cs:4900000,0.7416)
--(axis cs:5000000,0.774)
--(axis cs:5000000,0.88755)
--(axis cs:5000000,0.88755)
--(axis cs:4900000,0.86555)
--(axis cs:4800000,0.876)
--(axis cs:4700000,0.90355)
--(axis cs:4600000,0.85155)
--(axis cs:4500000,0.81355)
--(axis cs:4400000,0.85975)
--(axis cs:4300000,0.864)
--(axis cs:4200000,0.826)
--(axis cs:4100000,0.82775)
--(axis cs:4000000,0.8093)
--(axis cs:3900000,0.77105)
--(axis cs:3800000,0.7673)
--(axis cs:3700000,0.79355)
--(axis cs:3600000,0.7753)
--(axis cs:3500000,0.74355)
--(axis cs:3400000,0.74665)
--(axis cs:3300000,0.7442)
--(axis cs:3200000,0.7326)
--(axis cs:3100000,0.75465)
--(axis cs:3000000,0.7042)
--(axis cs:2900000,0.6773)
--(axis cs:2800000,0.66415)
--(axis cs:2700000,0.64975)
--(axis cs:2600000,0.63155)
--(axis cs:2500000,0.5895)
--(axis cs:2400000,0.53775)
--(axis cs:2300000,0.49905)
--(axis cs:2200000,0.5986)
--(axis cs:2100000,0.4595)
--(axis cs:2000000,0.4664)
--(axis cs:1900000,0.41955)
--(axis cs:1800000,0.30775)
--(axis cs:1700000,0.2286)
--(axis cs:1600000,0.2619)
--(axis cs:1500000,0.12865)
--(axis cs:1400000,0.0842)
--(axis cs:1300000,0.05485)
--(axis cs:1200000,0.05665)
--(axis cs:1100000,0.026)
--(axis cs:1000000,0.03155)
--(axis cs:900000,0.00555)
--(axis cs:800000,0.00355)
--(axis cs:700000,0.002)
--(axis cs:600000,0)
--(axis cs:500000,0)
--(axis cs:400000,0)
--(axis cs:300000,0)
--(axis cs:200000,0)
--(axis cs:100000,0)
--(axis cs:0,0)
--cycle;

\addplot [very thick, C1, mark=*, mark size=0, mark options={solid}]
table {%
0 0
100000 0
200000 0
300000 0
400000 0
500000 0
600000 0.016
700000 0.066
800000 0.046
900000 0.07
1000000 0.12
1100000 0.078
1200000 0.134
1300000 0.13
1400000 0.118
1500000 0.166
1600000 0.104
1700000 0.094
1800000 0.146
1900000 0.142
2000000 0.234
2100000 0.222
2200000 0.206
2300000 0.294
2400000 0.196
2500000 0.19
2600000 0.226
2700000 0.254
2800000 0.202
2900000 0.23
3000000 0.24
3100000 0.206
3200000 0.244
3300000 0.182
3400000 0.204
3500000 0.208
3600000 0.28
3700000 0.248
3800000 0.25
3900000 0.228
4000000 0.248
4100000 0.244
4200000 0.168
4300000 0.192
4400000 0.148
4500000 0.246
4600000 0.242
4700000 0.206
4800000 0.208
4900000 0.194
5000000 0.182
};
%\addlegendentry{sac}
\addplot [very thick, C0, mark=*, mark size=0, mark options={solid}]
table {%
0 0
100000 0
200000 0
300000 0
400000 0
500000 0
600000 0
700000 0
800000 0
900000 0
1000000 0.008
1100000 0.01
1200000 0.014
1300000 0.02
1400000 0.036
1500000 0.078
1600000 0.146
1700000 0.142
1800000 0.21
1900000 0.334
2000000 0.394
2100000 0.356
2200000 0.468
2300000 0.418
2400000 0.464
2500000 0.49
2600000 0.536
2700000 0.562
2800000 0.576
2900000 0.568
3000000 0.642
3100000 0.664
3200000 0.638
3300000 0.672
3400000 0.672
3500000 0.672
3600000 0.692
3700000 0.73
3800000 0.698
3900000 0.7
4000000 0.74
4100000 0.764
4200000 0.782
4300000 0.792
4400000 0.806
4500000 0.766
4600000 0.818
4700000 0.856
4800000 0.822
4900000 0.818
5000000 0.84
};
%\addlegendentry{vlearn}

\path [draw=C2, fill=C2, opacity=0.2]
(axis cs:0,0)
--(axis cs:0,0)
--(axis cs:204800,0)
--(axis cs:409600,0)
--(axis cs:614400,0)
--(axis cs:819200,0)
--(axis cs:1024000,0)
--(axis cs:1228800,0)
--(axis cs:1433600,0)
--(axis cs:1638400,0)
--(axis cs:1843200,0)
--(axis cs:2048000,0)
--(axis cs:2252800,0)
--(axis cs:2457600,0)
--(axis cs:2662400,0)
--(axis cs:2867200,0)
--(axis cs:3072000,0)
--(axis cs:3276800,0)
--(axis cs:3481600,0)
--(axis cs:3686400,0)
--(axis cs:3891200,0)
--(axis cs:4096000,0)
--(axis cs:4300800,0)
--(axis cs:4505600,0)
--(axis cs:4710400,0)
--(axis cs:4915200,0)
--(axis cs:5120000,0)
--(axis cs:5120000,0.004)
--(axis cs:5120000,0.004)
--(axis cs:4915200,0)
--(axis cs:4710400,0.002)
--(axis cs:4505600,0)
--(axis cs:4300800,0)
--(axis cs:4096000,0)
--(axis cs:3891200,0)
--(axis cs:3686400,0)
--(axis cs:3481600,0)
--(axis cs:3276800,0)
--(axis cs:3072000,0)
--(axis cs:2867200,0)
--(axis cs:2662400,0)
--(axis cs:2457600,0)
--(axis cs:2252800,0)
--(axis cs:2048000,0)
--(axis cs:1843200,0)
--(axis cs:1638400,0)
--(axis cs:1433600,0)
--(axis cs:1228800,0)
--(axis cs:1024000,0)
--(axis cs:819200,0)
--(axis cs:614400,0)
--(axis cs:409600,0)
--(axis cs:204800,0)
--(axis cs:0,0)
--cycle;

\path [draw=C7, fill=C7, opacity=0.2]
(axis cs:0,0)
--(axis cs:0,0)
--(axis cs:204800,0)
--(axis cs:409600,0)
--(axis cs:614400,0)
--(axis cs:819200,0)
--(axis cs:1024000,0)
--(axis cs:1228800,0)
--(axis cs:1433600,0)
--(axis cs:1638400,0)
--(axis cs:1843200,0)
--(axis cs:2048000,0)
--(axis cs:2252800,0)
--(axis cs:2457600,0)
--(axis cs:2662400,0)
--(axis cs:2867200,0.00445)
--(axis cs:3072000,0)
--(axis cs:3276800,0)
--(axis cs:3481600,0.002)
--(axis cs:3686400,0.008)
--(axis cs:3891200,0.00645)
--(axis cs:4096000,0)
--(axis cs:4300800,0.000450000000000002)
--(axis cs:4505600,0.01535)
--(axis cs:4710400,0.00445)
--(axis cs:4915200,0.026)
--(axis cs:5120000,0.02445)
--(axis cs:5120000,0.15545)
--(axis cs:5120000,0.15545)
--(axis cs:4915200,0.1271)
--(axis cs:4710400,0.07)
--(axis cs:4505600,0.1135)
--(axis cs:4300800,0.0573)
--(axis cs:4096000,0.06725)
--(axis cs:3891200,0.08955)
--(axis cs:3686400,0.09155)
--(axis cs:3481600,0.074)
--(axis cs:3276800,0.06555)
--(axis cs:3072000,0.04865)
--(axis cs:2867200,0.04265)
--(axis cs:2662400,0.0373)
--(axis cs:2457600,0.0231)
--(axis cs:2252800,0.012)
--(axis cs:2048000,0.01155)
--(axis cs:1843200,0.00155)
--(axis cs:1638400,0)
--(axis cs:1433600,0)
--(axis cs:1228800,0)
--(axis cs:1024000,0)
--(axis cs:819200,0)
--(axis cs:614400,0)
--(axis cs:409600,0)
--(axis cs:204800,0)
--(axis cs:0,0)
--cycle;

\addplot [very thick, C2, mark=*, mark size=0, mark options={solid}]
table {%
0 0
204800 0
409600 0
614400 0
819200 0
1024000 0
1228800 0
1433600 0
1638400 0
1843200 0
2048000 0
2252800 0
2457600 0
2662400 0
2867200 0
3072000 0
3276800 0
3481600 0
3686400 0
3891200 0
4096000 0
4300800 0
4505600 0
4710400 0
4915200 0
5120000 0
};
%\addlegendentry{trpl}
\addplot [very thick, C7, mark=*, mark size=0, mark options={solid}]
table {%
0 0
204800 0
409600 0
614400 0
819200 0
1024000 0
1228800 0
1433600 0
1638400 0
1843200 0
2048000 0
2252800 0
2457600 0.004
2662400 0.012
2867200 0.016
3072000 0.016
3276800 0.012
3481600 0.024
3686400 0.022
3891200 0.046
4096000 0.018
4300800 0.02
4505600 0.046
4710400 0.038
4915200 0.056
5120000 0.062
};
%\addlegendentry{ppo}

\path [draw=C3, fill=C3, opacity=0.2]
(axis cs:0,0)
--(axis cs:0,0)
--(axis cs:50000,0)
--(axis cs:100000,0.05765625)
--(axis cs:150000,0.21390625)
--(axis cs:200000,0.30625)
--(axis cs:250000,0.44375)
--(axis cs:300000,0.5125)
--(axis cs:350000,0.39109375)
--(axis cs:400000,0.575)
--(axis cs:450000,0.575)
--(axis cs:500000,0.59515625)
--(axis cs:550000,0.62921875)
--(axis cs:600000,0.6528125)
--(axis cs:650000,0.6653125)
--(axis cs:700000,0.56875)
--(axis cs:750000,0.636875)
--(axis cs:800000,0.65625)
--(axis cs:850000,0.7084375)
--(axis cs:900000,0.7125)
--(axis cs:950000,0.68890625)
--(axis cs:1000000,0.6778125)
--(axis cs:1050000,0.78265625)
--(axis cs:1100000,0.7153125)
--(axis cs:1150000,0.8125)
--(axis cs:1200000,0.75)
--(axis cs:1250000,0.80140625)
--(axis cs:1300000,0.85)
--(axis cs:1350000,0.77015625)
--(axis cs:1400000,0.84375)
--(axis cs:1450000,0.85)
--(axis cs:1500000,0.77921875)
--(axis cs:1550000,0.85625)
--(axis cs:1600000,0.661875)
--(axis cs:1650000,0.825)
--(axis cs:1700000,0.9)
--(axis cs:1750000,0.72015625)
--(axis cs:1800000,0.8625)
--(axis cs:1850000,0.85)
--(axis cs:1900000,0.85140625)
--(axis cs:1950000,0.87015625)
--(axis cs:1950000,0.93125)
--(axis cs:1950000,0.93125)
--(axis cs:1900000,0.95)
--(axis cs:1850000,0.9375)
--(axis cs:1800000,0.95484375)
--(axis cs:1750000,0.87984375)
--(axis cs:1700000,0.95484375)
--(axis cs:1650000,0.91109375)
--(axis cs:1600000,0.8909375)
--(axis cs:1550000,0.91875)
--(axis cs:1500000,0.89375)
--(axis cs:1450000,0.90625)
--(axis cs:1400000,0.89859375)
--(axis cs:1350000,0.8721875)
--(axis cs:1300000,0.875)
--(axis cs:1250000,0.86875)
--(axis cs:1200000,0.8596875)
--(axis cs:1150000,0.89859375)
--(axis cs:1100000,0.81875)
--(axis cs:1050000,0.90484375)
--(axis cs:1000000,0.82984375)
--(axis cs:950000,0.86109375)
--(axis cs:900000,0.86109375)
--(axis cs:850000,0.8875)
--(axis cs:800000,0.86875)
--(axis cs:750000,0.82359375)
--(axis cs:700000,0.83609375)
--(axis cs:650000,0.8375)
--(axis cs:600000,0.8346875)
--(axis cs:550000,0.7721875)
--(axis cs:500000,0.74375)
--(axis cs:450000,0.7125)
--(axis cs:400000,0.75828125)
--(axis cs:350000,0.6471875)
--(axis cs:300000,0.66109375)
--(axis cs:250000,0.5875)
--(axis cs:200000,0.519375)
--(axis cs:150000,0.41875)
--(axis cs:100000,0.13609375)
--(axis cs:50000,0)
--(axis cs:0,0)
--cycle;

\addplot [thick, C3, mark=*, mark size=0, mark options={solid}]
table {%
0 0
50000 0
100000 0.0875
150000 0.3375
200000 0.39375
250000 0.51875
300000 0.58125
350000 0.525
400000 0.66875
450000 0.64375
500000 0.6875
550000 0.7125
600000 0.75625
650000 0.7625
700000 0.71875
750000 0.7625
800000 0.79375
850000 0.83125
900000 0.79375
950000 0.8125
1000000 0.775
1050000 0.85625
1100000 0.78125
1150000 0.85625
1200000 0.8125
1250000 0.8375
1300000 0.8625
1350000 0.83125
1400000 0.875
1450000 0.875
1500000 0.85
1550000 0.8875
1600000 0.80625
1650000 0.8625
1700000 0.925
1750000 0.81875
1800000 0.9125
1850000 0.89375
1900000 0.90625
1950000 0.90625
};
% \addlegendentry{tdmpc2}

\end{axis}
\end{tikzpicture}
